# Supplementary material for: RoboNinja: Learning an Adaptive Cutting Policy for Multi-Material Objects
Source: arXiv:2302.11553 source file (2023-02-22)
Supplement: Supplementary file 1 [file appendix.tex]

\section{Appendix}
\label{sec:appendix}
